# Supplementary material for: Nonequilibrium plasmon emission drives ultrafast carrier relaxation dynamics in photoexcited graphene
Source: arXiv:1506.02525 source file (2015-09-30)
Supplement: Supplementary file 1 [file supplement.pdf]

# Nonequilibrium plasmon emission drives ultrafast carrier relaxation dynamics in photoexcited graphene - Supplementary Material

J. M. Hamm,[1,*] A. F. Page,[1] J. Bravo-Abad,[2] F. J. Garcia-Vidal,[2,3] and O. Hess[1,†]

[1] *Blackett Laboratory, Department of Physics, Imperial College London, London SW7 2AZ, United Kingdom*
[2] *Departamento de Física Teórica de la Materia Condensada and Condensed Matter Physics Center (IFIMAC), Universidad Autónoma de Madrid, E-28049 Madrid, Spain*
[3] *Donostia International Physics Center (DIPC), E-20018 Donostia/San Sebastian, Spain*

(Dated: September 30, 2015)

## I. THERMODYNAMIC RELATIONS

In quasi-equilibrium the carrier number and energy densities, $N$ and $U$, can be calculated by performing a sum over all electronic states weighted by the Fermi-Dirac distribution $f|_\mu^\vartheta(\epsilon_\mathbf{k})$ of electrons or holes, i.e.,

$$N(\mu,\vartheta) = \frac{g}{A}\sum_\mathbf{k} f|_\mu^\vartheta(\epsilon_\mathbf{k}) \tag{1}$$

$$U(\mu,\vartheta) = \frac{g}{A}\sum_\mathbf{k} \epsilon_\mathbf{k} f|_\mu^\vartheta(\epsilon_\mathbf{k}) \tag{2}$$

where $g = 4$ is the spin/valley degeneracy, $A$ the area of the graphene sheet, $\mu$ the chemical potential, and $\vartheta = k_B T_c$ the carrier temperature in energy units. The Dirac-cone approximation for the energy of the particles implies $\epsilon_\mathbf{k} = \hbar v_F|\mathbf{k}|$ for both electrons and holes. One then finds

$$N(\mu,\vartheta) = -\frac{2}{\pi}\frac{\vartheta^2 \mathrm{Li}_2\left(-e^{\mu/\vartheta}\right)}{(\hbar v_F)^2} \tag{3}$$

$$U(\mu,\vartheta) = -\frac{2}{\pi}\frac{2\vartheta^3 \mathrm{Li}_3\left(-e^{\mu/\vartheta}\right)}{(\hbar v_F)^2} \tag{4}$$

with $\mathrm{Li_n}$ being the $n$'th order polylogarithm. For the following we also require the derivatives of $N$ and $U$ with respect to $\mu$ and $\vartheta$. One may verify that

$$N_\mu(\mu,\vartheta) = \frac{\partial N(\mu,\vartheta)}{\partial\mu} = \frac{2}{\pi}\frac{\vartheta\log\left(1+e^{\mu/\vartheta}\right)}{(\hbar v_F)^2} \tag{5}$$

while the other derivatives can be expressed in form of algebraic relations, i.e. $N_\vartheta = \vartheta^{-1}(2N - \mu N_\mu)$, $U_\mu = 2N$ and $U_\vartheta = \vartheta^{-1}(3U - 2\mu N)$.

In quasi-equilibrium the carrier densities of the two components $N^\alpha(\mu^\alpha,\vartheta) = N(\mu^\alpha,\vartheta)$ and the total energy density $U(\mu^e,\mu^h,\vartheta) = U(\mu^e,\vartheta) + U(\mu^h,\vartheta)$ constitutes the set of extensive variables that describes the state of the carrier system. The partial derivatives of these quantities are the coefficients that connect the total differentials of the extensive variables with those of the intensive thermodynamic variables, i.e.,

$$\mathrm{d}N^\alpha = \frac{\partial N^\alpha}{\partial\mu^\alpha}\mathrm{d}\mu^\alpha + \frac{\partial N^\alpha}{\partial\vartheta}\mathrm{d}\vartheta \tag{6}$$

$$\mathrm{d}U = \frac{\partial U}{\partial\mu^e}\mathrm{d}\mu^e + \frac{\partial U}{\partial\mu^h}\mathrm{d}\mu^h + \frac{\partial U}{\partial\vartheta}\mathrm{d}\vartheta \tag{7}$$

Inverting the coefficient matrix yields,

$$\begin{aligned} c_U\mathrm{d}\vartheta &= \chi^e\mathrm{d}N^e + \chi^h\mathrm{d}N^h + \mathrm{d}U \\ \vartheta c_U\mathrm{d}\mu^\alpha &= \frac{\chi^\alpha}{N^\alpha}\left[\mu^\alpha N^\alpha - \chi^{\bar\alpha}N^{\bar\alpha} - \frac{3}{2}U\right]\mathrm{d}N^\alpha \\ &\quad + \chi^{\bar\alpha}\left[\mu^\alpha + \chi^\alpha\right]\mathrm{d}N^{\bar\alpha} + \left[\mu^\alpha + \chi^\alpha\right]\mathrm{d}U \end{aligned} \tag{8}$$

where $\bar\alpha = h$ $(e)$ for $\alpha = e$ $(h)$. The specific heat, $c_U = \vartheta^{-1}\left[3U + 2(\chi^e N^e + \chi^h N^h)\right]$, differs from the usual $c_U = U_\vartheta$ expression as it assumes the carrier density to be fixed (not the chemical potential). The coefficient $\chi^\alpha = -2N^\alpha/(\partial N^\alpha/\partial\mu)$ describes the change of temperature with carrier densities (for $U$ fixed).

## II. DERIVATION OF PLASMON RATES

In this section we present a derivation of the inter- and intraband plasmon absorption and emission rates according to Fermi's golden rule (FGR). Consider complex-frequency roots $\omega(q) = \omega_\mathrm{pl}(q) - i\gamma_\mathrm{pl}(q)$ of the dynamic dielectric function in random-phase approximation, i.e.,

$$\varepsilon_\mathrm{RPA}(q,\omega) = 1 - V_q\Pi(q,\omega) = 0 \tag{9}$$

where $\Pi(q,\omega)$ is the irreducible polarizability and $V_q = e^2/(2\varepsilon_0 q)$ the bare Coulomb potential. While $\omega_\mathrm{pl}(q)$ defines the plasmon dispersion, $\gamma_\mathrm{pl}(q)$ represents the net decay rate of the field amplitude due to stimulated processes, i.e. stimulated absorption minus emission. A first order Taylor expansion of Eq. (9) gives

$$\gamma_\mathrm{pl}(q) \approx -V_q \left.\frac{\mathrm{Im}[\Pi(q,\omega)]}{\frac{\partial\mathrm{Re}[\varepsilon_\mathrm{RPA}(q,\omega)]}{\partial\omega}}\right|_{\omega=\omega_\mathrm{pl}(q)} . \tag{10}$$

The net decay of the plasmon number due to stimulated processes,

$$\frac{\partial n_\mathrm{pl}}{\partial t} = -\gamma_\mathrm{pl}^\mathrm{stim} n_\mathrm{pl} , \tag{11}$$

* j.hamm@imperial.ac.uk
† o.hess@imperial.ac.uk

is associated with a decay rate $\gamma_{\rm pl}^{\rm stim} = 2\gamma_{\rm pl}$, as $\gamma_{\rm pl}$ describes a field decay while $\gamma_{\rm pl}^{\rm stim}$ is intensity related. Inserting the Lindhard formula for the polarizability and evaluating the Lorentz pole results in the following FGR expression for the net stimulated absorption process [1],

$$\gamma_{\rm pl}^{\rm stim} = \frac{2\pi}{\hbar}\frac{g}{A}\sum_{s,s'=\pm}\sum_{\mathbf{k}} V_q \left.\frac{\hbar\delta(\hbar\omega + \epsilon^s_{\mathbf{k}} - \epsilon^{s'}_{\mathbf{k+q}})}{\frac{\partial \mathrm{Re}[\varepsilon_{\rm RPA}(q,\omega)]}{\partial\omega}}\right|_{\omega=\omega_{\rm pl}(q)}, \times M^{ss'}_{\mathbf{k},\mathbf{k+q}}\left[f(\epsilon^{s'}_{\mathbf{k+q}}) - f(\epsilon^s_{\mathbf{k}})\right] \tag{12}$$

where $M^{ss'}_{\mathbf{k},\mathbf{k}'}$ denotes the square of the matrix element. The expression above is in agreement with [2]. For brevity of the following argument we define $f = f(\epsilon^s_{\mathbf{k}})$ and $f' = f(\epsilon^{s'}_{\mathbf{k+q}})$. The net stimulated rate above can be split into absorption and emission contributions using the formal identity $f' - f = f'(1-f) - f(1-f')$. Using this prescription we split $\gamma_{\rm pl}^{\rm stim} = \gamma_{\rm pl}^{-} - \gamma_{\rm pl}^{+}$, where $\gamma_{\rm pl}^{\pm}$ are the emission and absorption rates. Note, that Eq. (12) still contains a sum over inter- and intraband transitions, so that $\gamma_{\rm pl}^{\pm} = \sum_\lambda \gamma_{{\rm pl},\lambda}^{\pm}$ with $\lambda = ee, hh, eh, he$. Evaluating the sum over $k$ (see [1] for details) gives

$$\gamma_{{\rm pl},eh}^{\pm}(q) \approx \alpha_g \left.\frac{2\theta(\omega - v_F q)}{\sqrt{\left(\frac{\omega}{v_F q}\right)^2 - 1}}\frac{K^{\pm}_{eh}(q,\omega)}{\frac{\partial \mathrm{Re}[\varepsilon(q,\omega)]}{\partial\omega}}\right|_{\omega=\omega_{\rm pl}(q)}, \tag{13}$$

for the interband emission and absorption. Here $\alpha_g = \alpha_f c/v_F$ is the finestructure constant of graphene and $\varepsilon(q,\omega)$ the dielectric function. The integrals $K^{\pm}_{eh}$ are given by

$$K^{+}_{eh}|^{\vartheta}_{\mu^e,\mu^h}(q,\omega) = \int_{-1}^{+1} \mathrm{d}u\,\sqrt{1-u^2} \times f|^{\vartheta}_{\mu^e}(\hbar(\omega + v_F q u)/2) \times f|^{\vartheta}_{\mu^h}(\hbar(\omega - v_F q u)/2) \tag{14}$$

and

$$K^{-}_{eh}|^{\vartheta}_{\mu^e,\mu^h}(q,\omega) = \int_{-1}^{+1} \mathrm{d}u\,\sqrt{1-u^2} \times [1 - f|^{\vartheta}_{\mu^e}(\hbar(\omega + v_F q u)/2)] \times [1 - f|^{\vartheta}_{\mu^h}(\hbar(\omega - v_F q u)/2)] \tag{15}$$

Finally, we note, that the rates $\gamma_{{\rm pl},eh}^{\pm}(q)$ relate to the emission/absorption spectra via

$$\Gamma^{\pm}_{{\rm pl},eh}(\omega) = D_{\rm pl}(\omega)\gamma^{\pm}_{{\rm pl},eh}(q_{\rm pl}(\omega)) \tag{16}$$

where $D_{\rm pl}(\omega) = (2\pi)^{-1} q_{\rm pl}(\omega)\partial q_{\rm pl}(\omega)/d\omega$ is the density of states of plasmons whose wavevector dispersion is given by $q_{\rm pl}(\omega)$.

## III. RATES AND DENSITY OF INTRINSIC OPTICAL PHONONS

In following we derive the analytical equations for the inter- and intraband phonon emission and absorption rates from the integral equations. For the interband processes one finds [3, 4]

$$\Gamma^{+}_{\circ,eh} = \kappa_\circ \int_{-\epsilon_\circ/2}^{+\epsilon_\circ/2} \mathrm{d}\epsilon'\,[(\epsilon_\circ/2)^2 - (\epsilon')^2)] \times f|^{\vartheta}_{\mu^e}(\epsilon_\circ/2 + \epsilon') f|^{\vartheta}_{\mu^h}(\epsilon_\circ/2 - \epsilon') \tag{17}$$

and

$$\Gamma^{-}_{\circ,eh} = \kappa_\circ \int_{-\epsilon_\circ/2}^{+\epsilon_\circ/2} \mathrm{d}\epsilon'\,[(\epsilon_\circ/2)^2 - (\epsilon')^2)] \times [1 - f|^{\vartheta}_{\mu^e}(\epsilon_\circ/2 + \epsilon')][1 - f|^{\vartheta}_{\mu^h}(\epsilon_\circ/2 - \epsilon')] \tag{18}$$

where $\kappa_\circ = 2\beta_\circ^2/[\pi\rho_m(\hbar v_F)^4]$ is a constant that contains the deformation potential $\beta_\circ$ of the optical phonon branch and the mass-density $\rho_m = 7.6 \times 10^{-7}\mathrm{kg/m}^2$ of graphene. For the deformation potential we use values of $\beta_{\Gamma O} = \beta_{KO} = 45\,\mathrm{eV/nm}$ and $\beta_{KA} = 2/3 \times 35\,\mathrm{eV/nm}$ in accordance with [3]. Using these values the intrinsic scattering times $\tau_\circ = 1/\eta_\circ$ associated with the scattering processes are found as $\tau_{\Gamma O} = \tau_{KO} = 0.684\,\mathrm{ps}$ and $\tau_{KA} = 2.54\,\mathrm{ps}$, respectively. After splitting the integration into intervals $[-\epsilon_\circ/2, 0]$ and $[0, \epsilon_\circ/2]$ it is possible to carry out the integration to obtain

$$\Gamma^{\pm}_{\circ,eh} = \mp\eta_\circ \frac{\tilde{N}_\circ(\mu^e,\vartheta) + \tilde{N}_\circ(\mu^h,\vartheta)}{\exp\left[\mp\frac{(\mu^e+\mu^h)-\epsilon_\circ}{\vartheta}\right] - 1} \tag{19}$$

with $\eta_\circ = \frac{\pi}{2}(\hbar v_F)^2\epsilon_\circ\kappa_\circ$. The effective densities $\tilde{N}_\circ(\mu,\vartheta)$ quantifies the number of carriers that participate in the interband scattering process. It is given by the following closed-form expression

$$\begin{aligned}\tilde{N}_\circ(\mu,\vartheta) = & N(\mu,\vartheta) - N(\epsilon_\circ - \mu,\vartheta) \\ & + \frac{\epsilon_\circ}{4}\left[N_\mu(\epsilon_\circ/2 - \mu,\vartheta) - N_\mu(\mu - \epsilon_\circ/2,\vartheta)\right] \\ & - \epsilon_\circ^{-1}\left[U(\mu,\vartheta) - U(\epsilon_\circ - \mu,\vartheta)\right] \\ & - \epsilon_\circ^{-1}\left[U(\epsilon_\circ/2 - \mu,\vartheta) - U(\mu - \epsilon_\circ/2,\vartheta)\right]\end{aligned} \tag{20}$$

with $N_\mu = \partial N/\partial\mu$. The integral expressions for the intraband emission and absorption rates are [4]

$$\Gamma^{+}_{\circ,\alpha\alpha} = \kappa_\circ \int_{\epsilon_\circ}^{\infty} \mathrm{d}\epsilon'\,\epsilon'[\epsilon' - \epsilon_\circ] \times f|^{\vartheta}_{\mu^\alpha}(\epsilon')[1 - f|^{\vartheta}_{\mu^\alpha}(\epsilon' - \epsilon_\circ)] \tag{21}$$

and

$$\Gamma^{-}_{\circ,\alpha\alpha} = \kappa_\circ \int_{\epsilon_\circ}^{\infty} \mathrm{d}\epsilon'\,\epsilon'[\epsilon' - \epsilon_\circ] \times [1 - f|^{\vartheta}_{\mu^\alpha}(\epsilon')] f|^{\vartheta}_{\mu^\alpha}(\epsilon' - \epsilon_\circ) \tag{22}$$

Again, one can carry out the integration to find the analytical result

$$\Gamma^{\pm}_{\circ,eh} = \mp\eta_\circ \frac{\tilde{N}_\circ(\mu^e,\vartheta) + \tilde{N}_\circ(\mu^h,\vartheta)}{\exp\left[\mp\frac{(\mu^e+\mu^h)-\epsilon_\circ}{\vartheta}\right] - 1} \tag{23}$$

given in the main text, which depends on the effective carrier density

$$\begin{aligned}\bar{N}_\circ(\mu,\vartheta) =& N(\mu,\vartheta) - N(\mu-\epsilon_\circ,\vartheta) \\ &+ \epsilon_\circ^{-1}\left[U(\mu,\vartheta) - U(\mu-\epsilon_\circ,\vartheta)\right]\end{aligned} \tag{24}$$

The carrier recombination and generation rates $\Gamma^{\pm}_{\circ,\lambda}$ relate to the phonon emission/absorption rates $\gamma^{\pm}_{\circ,\lambda}$ via $\Gamma^{\pm}_{\circ,\lambda} = M_{\circ,\lambda}\gamma^{\pm}_{\circ,\lambda}$. The phonon densities $M_{\circ,\lambda}$ are required to translate the net emission rate $R_{\circ,\lambda}$ (in units $m^{-2}s^{-1}$) into a rate $\partial n_\circ/\partial t$ (in $s^{-1}$). One can associate $M_{\circ,\lambda}$ with the area in momentum space into which phonons are emitted by the respective scattering process [CITE: ?]. Taking into account a degeneracy of 2 for both the ΓO and KO phonons one finds $M_{\circ,\lambda} = 1/(2\pi)[q^2_{\max} - q^2_{\min}]$. For the interband scattering the integral over the carrier energy has a range $[0,\epsilon_\circ]$. Momentum conservation dictates that $q_{\min} = 0$ and $q_{\max} = \epsilon_\circ/(\hbar v_F)$. In contrast, optical phonons emitted via intraband scattering have a minimum wavevector of $q_{\min} = \epsilon_\circ/(\hbar v_F)$ but no hard cut-off for their maximum wavevector. Instead, phonon emission is limited by the lack of carriers at higher energies due to the rapid decay of the Fermi-functions for energies above the respective chemical potentials [4]. It is clear from Eq. (21) that while the density of energy states increases with $\epsilon(\epsilon - \hbar\omega_\circ)$ the intraband emission becomes increasingly ineffective for higher energies, due to the exponential decay of the product of the Fermi-functions. To estimate the cut-off energy $\epsilon_{\text{cut}}$ we first note that $f(\epsilon-\mu^\alpha,\vartheta)\left[1 - f(\epsilon-\epsilon_\circ-\mu^\alpha,\vartheta)\right]$ peaks at $\epsilon = \mu + \epsilon_\circ/2$ with a value of $1/(1+\exp[\epsilon_\circ/(2\vartheta)])^2$. Using some basic algebra we estimate the energy at which the function has decayed to a $n$'th of the peak value with

$$\begin{aligned}\epsilon_{\text{cut}} \approx& \mu^\alpha \\ &+ \vartheta \log\left[(n-1)\left\{1 + e^{\epsilon_\circ/\vartheta}\right\} + 2ne^{\epsilon_\circ/(2\vartheta)}\right]\end{aligned} \tag{25}$$

The value of $n$ remains somewhat arbitrary. It can be shown that $n$ just needs to be large enough to ensure that the Fermi-functions decayed sufficiently strong compensating for the steady increase in the density of states, which pushes the cut-off to higher $k$ values. Considering temperatures of thousands of Kelvin and chemical potentials down to 0.05 eV we find that $n = 50$ provides an excellent approximation for energy cut-off.


[1] A. F. Page, F. Ballout, O. Hess, and J. M. Hamm, Phys. Rev. B **91**, 75404 (2015).

[2] F. Rana, J. H. Strait, H. Wang, and C. Manolatou, Phys. Rev. B **84**, 045437 (2011).

[3] F. Rana, P. A. George, J. H. Strait, J. M. Dawlaty, S. Shivaraman, M. Chandrashekhar, and M. G. Spencer, Phys. Rev. B **79**, 115447 (2009).

[4] H. Wang, J. H. Strait, P. A. George, S. Shivaraman, V. B. Shields, M. Chandrashekhar, J. Hwang, F. Rana, M. G. Spencer, C. S. Ruiz-Vargas, and J. Park, Appl. Phys. Lett. **96**, 081917 (2010).
